# Supplementary material for: Pump-Threshold-Free Frequency Comb via Cavity Floquet Engineering
Source: arXiv:2504.05877 ancillary file (2026-04-25)
Supplement: Supplementary file 1 [file Supplementary_Material_Threshold_less_Floquet_Comb.pdf]

# Supplementary Information for “Threshold-less and Flexibly Tunable Frequency Comb via Floquet Engineering”

Sihan Wang,<sup>1,2,3,4</sup> Cheng Wang,<sup>5</sup> Matthijs H. J. de Jong,<sup>5</sup> Laure Mercier de Lépinay,<sup>5</sup> Jingwei Zhou,<sup>3,4,\*</sup> Mika A. Sillanpää,<sup>5</sup> and Yulong Liu<sup>1,2,†</sup>

<sup>1</sup>*Beijing academy of quantum information sciences, Beijing, 100193, China*

<sup>2</sup>*Beijing Key Laboratory of Fault-Tolerant Quantum Computing, Beijing 100193, China*

<sup>3</sup>*Hefei National Research Center for Physics Sciences at Microscale,  
University of Science and Technology of China, Hefei 230026, China*

<sup>4</sup>*CAS Key Laboratory of Microscale Magnetic Resonance,  
University of Science and Technology of China, Hefei 230026, China*

<sup>5</sup>*QTF Centre of Excellence, Department of Applied Physics, Aalto University, FI-00076 Aalto, Finland*

(Dated: April 8, 2025)

## Contents

|                                                            |    |
|------------------------------------------------------------|----|
| I. Floquet Cavity                                          | 1  |
| A. Two classic examples                                    | 2  |
| 1. A Planar Pendulum Periodic Modulation its Length of Rod | 2  |
| 2. LC CircuitS with Time-modulated Capacitor               | 3  |
| B. Quantum theory of Floquet cavity                        | 4  |
| C. Dynamics equation of Floquet cavity                     | 6  |
| II. Floquet Cavity Frequency Comb                          | 7  |
| A. Dynamics equation with pump tone                        | 7  |
| B. Input-output theory                                     | 10 |
| III. Microwave Optomechanical Device and Characterization  | 10 |
| A. Sample fabrication                                      | 10 |
| B. Detailed experimental setup                             | 11 |
| C. Parameter characterization                              | 11 |
| IV. Self-induced oscillations by blue-detuned driving      | 13 |
| V. Extended Data                                           | 14 |
| A. Frequency shift caused by equilibrium position shift    | 14 |
| B. The self-induced oscillation regime                     | 15 |
| C. Detailed Floquet Frequency Comb                         | 15 |
| References                                                 | 15 |

## Supplementary Note I Floquet Cavity

As is introduced in the main text, the term “Floquet” is associated with time periodicity. More specifically, in a classical context, Floquet theory was introduced to describe the behavior of a set of linear differential equations with time-periodic coefficients, originally arising from the problem of stability of periodic orbits in classical mechanics. In the quantum domain, where the linearity of the Schrödinger equation is inherent, Floquet theory applies whenever the Hamiltonian governing the system is time-periodic,  $\hat{H}(t) = \hat{H}(t + T)$ , where  $T$  is the period.

---

\* [zhoujw@ustc.edu.cn](mailto:zhoujw@ustc.edu.cn)

† [liuy1@baqis.ac.cn](mailto:liuy1@baqis.ac.cn)

### A. Two classic examples

Before the derivation of the Floquet cavity and frequency comb, several well-known examples are mentioned in the main text. Here, we provide a brief analysis and introduction to demonstrate the capability of Floquet engineering in constructing multi-frequency components [1].

#### 1. A Planar Pendulum Periodic Modulation its Length of Rod

As shown in Fig. S1a, the dynamics of the system can be analyzed using classical equations of motion in a reference frame centered at the fixed point, where the Y-axis is vertical and the X-axis is horizontal. The position of the mass  $m$  in this frame is described by the generalized coordinates  $x(t)$  and  $y(t)$ , as follows:

$$\begin{cases} x(t) = l(t) \sin \theta(t) \\ y(t) = -l(t) \cos \theta(t) \end{cases} \Rightarrow \begin{cases} \dot{x}(t) = \dot{l} \sin \theta + l \dot{\theta} \cos \theta \\ \dot{y}(t) = -\dot{l} \cos \theta + l \dot{\theta} \sin \theta \end{cases} \quad (\text{S1})$$

Here,  $l(t)$  is the time-dependent length of the system, and  $\theta(t)$  represents the angular displacement measured from downward vertical. The Hamiltonian is defined as:

$$H_{\text{lab}}(\theta, p_\theta, t) = \frac{p_\theta^2}{2ml^2} - \frac{m}{2} \dot{l}^2 - mgl \cos \theta. \quad (\text{S2})$$

where  $p_\theta$  is the canonical momentum conjugate, and  $g$  represents the gravitational acceleration. And from the Hamilton's equations, we can obtain the second-order equation of motion for  $\theta$ :

$$\frac{d^2 \theta}{dt^2} = -\frac{g}{l} \sin \theta - \frac{2\dot{l}}{l} \dot{\theta} \quad (\text{S3})$$

This equation accounts for both the gravitational restoring force and a damping term proportional to  $\dot{l}$ , which arises from the time-dependent nature of the length  $l(t)$ . To model a system with a time-dependent length, we assume:

$$l(t) = l_0 + l_m \sin(\Omega t) = l_0(1 + \lambda \sin(\Omega t)) \quad (\text{S4})$$

where  $l_0$  is the equilibrium length,  $l_m$  is the modulation length,  $\lambda$  is the relative modulation length, and  $\Omega$  is the frequency of oscillation. Substituting this expression into the equation of motion, we obtain:

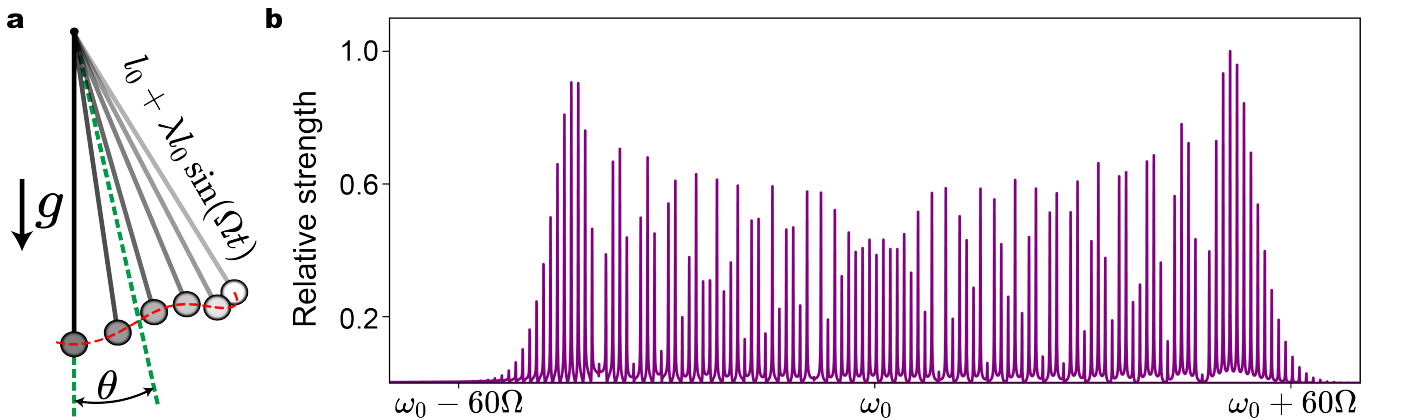

FIG. S1. **a** Schematic of the modulated pendulum. **b** Example of the superposition of multiple frequencies generated by the modulated planar pendulum. Here,  $\lambda = 0.1, \Omega = 0.001\omega_0$ . The relative strengths are normalized to the strongest frequency component.

$$\ddot{\theta} + \underbrace{\frac{g}{l_0 + \lambda l_0 \sin(\Omega t)}}_{\text{time-varying gravitational term}} \sin \theta + \underbrace{\frac{2\lambda l_0 \Omega \cos(\Omega t)}{l_0 + \lambda l_0 \sin(\Omega t)}}_{\text{parametric damping/excitation}} \dot{\theta} = 0 \quad (\text{S5})$$

For small oscillations ( $\sin \theta \approx \theta$ ), the equation is similar to the Mathieu equation for parametric excitation. The system exhibits chaotic behavior under the driving amplitude exceeds  $\lambda \sim 1$  or parametric resonance  $\Omega \approx 2\omega_0$  ( $\omega_0 = \sqrt{g/l_0}$ ). For  $\Omega \ll \omega_0$ , we can show its ability to generate sidebands, a numerical demonstration is shown in Fig. S1b.

## 2. LC CircuitS with Time-modulated Capacitor

The current dynamics in an LC circuit with time-dependent capacitance can be described by the differential equation:

$$\frac{d^2 I}{dt^2} + \frac{1}{L(C + C_m \cos(\Omega t))} I = 0, \quad (\text{S6})$$

where  $L$  is the inductance,  $C$  is the static capacitance,  $C_m$  is the modulation amplitude, and  $\Omega$  is the modulation frequency. Under the assumption of small capacitance modulation ( $C_m \ll C$ ), the time-dependent term can be expanded using a first-order Taylor approximation:

$$\frac{1}{C + C_m \cos(\Omega t)} \approx \frac{1}{C} \left( 1 - \frac{C_m}{C} \cos(\Omega t) \right). \quad (\text{S7})$$

Substituting Equation (S7) into Equation (S6) yields:

$$\frac{d^2 I}{dt^2} + \frac{1}{LC} \left( 1 - \frac{C_m}{C} \cos(\Omega t) \right) I = 0. \quad (\text{S8})$$

Defining the natural frequency of the unmodulated system as  $\omega_0^2 = 1/(LC)$  and introducing the parametric modulation strength  $\lambda = -C_m \omega_0^2 / C$ , Equation (S8) reduces to the canonical form of the Mathieu equation:

$$\frac{d^2 I}{dt^2} + (\omega_0^2 + \lambda \cos(\Omega t)) I = 0. \quad (\text{S9})$$

This equivalence demonstrates that the system exhibits parametric resonance behavior characteristic of Mathieu-type equations. From this form, the instantaneous angular frequency can be identified as

$$\omega(t) = \omega_0 \sqrt{1 - \frac{C_m}{C} \cos(\Omega t)}. \quad (\text{S10})$$

Applying a first-order approximation for small  $C_m/C$ , we obtain

$$\omega(t) \approx \omega_0 \left( 1 - \frac{C_m}{2C} \cos(\Omega t) \right). \quad (\text{S11})$$

Thus, the frequency modulation can be expressed as

$$\omega(t) = \omega_0 + A \cos(\Omega t), \quad (\text{S12})$$

where the modulation amplitude is given by  $A = -(C_m/2C)\omega_0$ . This result indicates that the system undergoes a harmonic modulation of its resonance frequency with an amplitude proportional to  $C_m/C$ . For inductance modulation, the result is similar.

### B. Quantum theory of Floquet cavity

As mentioned in the main text and methods, for a general Floquet cavity, we consider the following time-dependent Hamiltonian that is periodic in time,  $H(t) = H(t + T)$  with  $\Omega = 2\pi/T$ :

$$H(t) = (\omega_0 + A \cos \Omega t + \phi) a^\dagger a, \quad (\text{S13})$$

where  $\omega_0$  is the intrinsic frequency,  $A$  is the modulation strength,  $\Omega$  is the modulation frequency, and  $\phi$  is the inconsequential initial phase of the modulation which can be set to zero without loss of generality. Analogous to the classical case, we here consider  $\Omega \ll \omega_0$  in order to avoid parametric resonance. The quantum state  $|\psi, t\rangle$  of this closed system  $H(t)$  is governed by the Schrödinger equation ( $\hbar = 1$ ),

$$i\partial_t |\psi, t\rangle = H(t) |\psi, t\rangle. \quad (\text{S14})$$

According to the Floquet's theorem [cite], the general form of the solution  $|\psi_\alpha, t\rangle$  to the Eq.S14 can be written as

$$|\psi_\alpha, t\rangle = e^{-i\varepsilon_\alpha t} |u_\alpha, t\rangle, |u_\alpha, t\rangle = |u_\alpha, t + T\rangle, \quad (\text{S15})$$

The  $|\psi_\alpha, t\rangle$  is referred to as steady-state solution. So the Hamiltonian can be represented as a diagonal matrix  $H(t) = \sum_n h_n(t) |n\rangle\langle n|$  under the Fock basis  $\{|n\rangle\}$ , with matrix elements of  $h_n(t) = n(\omega_0 + A \cos \Omega t)$ . Thus, the Schrödinger equation

$$i\partial_t |\psi, t\rangle = \sum_n n(\omega_0 + A \cos \Omega t) |n\rangle\langle n| |\psi, t\rangle \quad (\text{S16})$$

can be simplified as

$$i\partial_t \psi_n(t) = n(\omega_0 + A \cos \Omega t) \psi_n(t) \quad (\text{S17})$$

here  $\psi_n(t) = \langle n | \psi, t \rangle$ . The solution to the Eq.S17 that is not difficult to solve is

$$\begin{aligned} \psi_n(t) &= c e^{-i \int_0^t h_n(t) dt} \\ &= c e^{-in\omega_0 t} e^{-in \frac{A}{\Omega} \sin \Omega t} \end{aligned} \quad (\text{S18})$$

with  $c$  the indeterminate constant. Combined with Eq. S15, the steady-state solution of Eq. S16 is expressed as

$$\begin{aligned} |\psi_n, t\rangle &= e^{-in\omega_0 t} |u_n, t\rangle \\ |u_n, t\rangle &= e^{-in \frac{A}{\Omega} \sin \Omega t} |n\rangle \end{aligned} \quad (\text{S19})$$

We can check that the  $|u_n, t\rangle$  satisfies  $|u_n, t + T\rangle = |u_n, t\rangle$  with  $T = 2\pi/\Omega$ . Defining

$$\begin{aligned} |u_{nm}, t\rangle &= |u_n, t\rangle e^{im\Omega t} \\ &= u_{nm}(t) |n\rangle \\ u_{nm}(t) &= e^{-in \frac{A}{\Omega} \sin \Omega t} e^{im\Omega t}, \end{aligned} \quad (\text{S20})$$

which satisfies

$$H_F |u_{nm}, t\rangle = \varepsilon_{nm} |u_{nm}, t\rangle. \quad (\text{S21})$$

Here, we define Brillouin regions over the frequency domain, where the single Brillouin region have a width of  $\Omega$ , and the different Brillouin regions are represented by the index  $m$ , called the Floquet index. Here  $H_F = H(t) - i\partial_t$  is known as the Floquet Hamiltonian,  $|u_{nm}, t\rangle$  represents the time-periodic Floquet state, and the quasi-energy is given

by  $\varepsilon_{nm} = n\omega_0 + m\Omega$ , where  $m$  ranges from negative to positive infinity. This implies that the entire Floquet cavity functions as a giant-mode cavity with  $2m$  modes. The  $|u_n, t\rangle$  can also be written as  $|u_{n0}, t\rangle$ . Under the complete base vector set  $\{|n_m\rangle\rangle\}$  with  $|n_m\rangle = |n\rangle e^{im\Omega t}$ , the matrix elements of the Floquet Hamiltonian are

$$\langle\langle n_m | H_F | n'_{m'} \rangle\rangle = \langle n | H^{[m-m']} | n' \rangle + m' \Omega \delta_{mm'} \delta_{nn'}, \quad (\text{S22})$$

where  $H^{[l]}$  is the Fourier component of  $H(t)$ . Since

$$\begin{aligned} H(t) &= \sum_n n (\omega_0 + A \cos \Omega t) |n\rangle \langle n| \\ &= \sum_n n \left( \Omega_0 + \frac{A}{2} e^{i\Omega t} + \frac{A}{2} e^{-i\Omega t} \right) |n\rangle \langle n| \\ &= \sum_l H^{[l]} e^{il\Omega t} \end{aligned} \quad (\text{S23})$$

where  $H^{[0]} = \sum_n n\omega_0 |n\rangle \langle n|$ ,  $H^{[\pm 1]} = \sum_n n \frac{A}{2} |n\rangle \langle n|$ , and  $H^{[l]} = 0$  for  $|l| > 1$ . Thus, the Eq. S22 can be further expressed as

$$\langle\langle n_m | H_F | n'_{m'} \rangle\rangle = \delta_{nn'} \left( n\omega_0 \delta_{mm'} + n \frac{A}{2} \delta_{m, m' \pm 1} \right) + m' \Omega \delta_{mm'} \delta_{nn'}, \quad (\text{S24})$$

Obviously,  $H_F$  is a block diagonal form about  $n$ , and we write the projection of  $H_F$  in subspace  $\{|n_m\rangle\rangle\}$  with fixed  $n$  as  $H_F^{(n)}$ ,

$$H_F^{(n)} = \begin{bmatrix} \ddots & \vdots & \vdots & \vdots & \ddots \\ \cdots & n\omega_0 - \Omega & n\frac{A}{2} & 0 & \cdots \\ \cdots & n\frac{A}{2} & n\omega_0 & n\frac{A}{2} & \cdots \\ \cdots & 0 & n\frac{A}{2} & n\omega_0 + \Omega & \cdots \\ \ddots & \vdots & \vdots & \vdots & \ddots \end{bmatrix}, \quad (\text{S25})$$

which satisfies  $H_F^{(n)} |u_{nm}\rangle\rangle = \varepsilon_{nm} |u_{nm}\rangle\rangle$  according to the Eq. S21. We will write  $|u_{nm}, t\rangle$  in the form of Fourier expansion  $|u_{nm}, t\rangle = \sum_l u_{nm}^{[l]} e^{il\Omega t} |n\rangle = \sum_l u_{nm}^{[l]} |n_l, t\rangle$ , so we have  $|u_{nm}\rangle\rangle = \sum_l u_{nm}^{[l]} |n_l\rangle\rangle$ . This means that  $u_{nm}^{[l]}$  can be obtained by diagonalizing the Hamiltonian  $H_F^{(n)}$ . In this Floquet cavity model,  $u_{nm}(t)$  can be easily solved, so  $u_{nm}^{[l]}$  can be directly given based on the expression of  $u_{nm}(t)$ . However, for general cases, the solution of  $u_{nm}^{[l]}$  requires diagonalization of  $H_F$ .

Assuming the initial state of the system is  $|\psi, t=0\rangle = |n\rangle$ , then  $|\psi, t\rangle$  will be in steady state with quasienergy  $n\omega_0$ , i.e.,  $|\psi, t\rangle = |\psi_n, t\rangle = e^{-i\omega_0 t} |u_n, t\rangle$ . The time-averaged expectation value of the energy is

$$\begin{aligned} E &= \frac{1}{T} \int_0^T dt \langle \psi_n, t | H(t) | \psi_n, t \rangle \\ &= \frac{1}{T} \int_0^T dt \langle u_n, t | H(t) | u_n, t \rangle \\ &= \langle \langle u_{n0} | H(t) | u_{n0} \rangle \rangle \\ &= \langle \langle u_{n0} | H_F + i\partial_t | u_{n0} \rangle \rangle \\ &= n\omega_0 + \langle \langle u_{n0} | i\partial_t | u_{n0} \rangle \rangle \end{aligned} \quad (\text{S26})$$

By substituting into the Floquet Hamiltonian, we obtain:

$$\begin{aligned}
E &= n\omega_0 + i \sum_{ll'} u_{n0}^{[l]} u_{n0}^{*[l']} \langle n_l' | \partial_t | n_l \rangle \\
&= n\omega_0 - \sum_l |u_{n0}^{[l]}|^2 l\omega \\
&= \sum_l (n\omega_0 - l\omega) |u_{n0}^{[l]}|^2 \\
&= \sum_m \varepsilon_{nm} |u_{n0}^{[-m]}|^2
\end{aligned} \tag{S27}$$

which can be interpreted to mean that when the system is in the quantum state  $|\psi_n, t\rangle = e^{-i\varepsilon_{nn}t} |u_n, t\rangle$ , the probability of energy  $\varepsilon_{nm}$  occurring is  $|u_{n0}^{[-m]}|^2$ . Noting that  $\sum_m |u_{n0}^{[-m]}|^2 = 1$  due to the normalization of  $|u_{n0}\rangle$ . For the single-excitation situation with  $n = 1$ ,  $\varepsilon_{n=1,m} = \omega_0 + m\omega$ .

### C. Dynamics equation of Floquet cavity

To better analyze and display the time-domain and frequency-domain information of the Floquet cavity's giant mode, we studied the dynamics equation for the evolution of the complex amplitude  $a(t)$ .

$$\dot{a}(t) = \left[ -\frac{\kappa}{2} - i(\omega_0 + A \cos(\Omega t)) \right] a(t), \tag{S28}$$

where  $\kappa$  is the total decay rate. To simplify the problem, we perform a transformation of the form:

$$a(t) = e^{\frac{-iA \sin(\Omega t)}{\Omega}} c(t), \tag{S29}$$

which introduces a time-dependent phase factor  $e^{\frac{-iA \sin(\Omega t)}{\Omega}}$ . Substituting this into the dynamics equation leads to a simplified equation for  $c(t)$ :

$$\dot{c}(t) = \left( -\frac{\kappa}{2} - i\omega_0 \right) c(t). \tag{S30}$$

The solution to this equation is straightforward:

$$c(t) = c_0 e^{(-\frac{\kappa}{2} - i\omega_0)t}, \tag{S31}$$

where  $c_0$  depends on the initial conditions. Substituting this back into the expression for  $a(t)$ , we obtain:

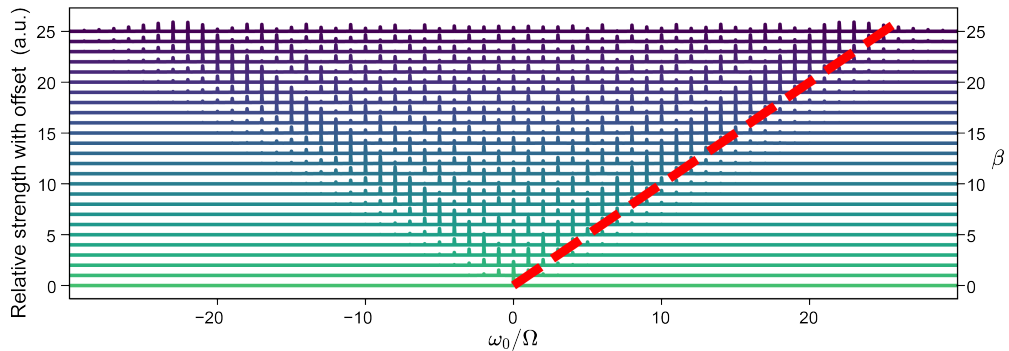

FIG. S2. The mode distribution of the cavity as a function of  $\beta$ . For each  $\beta$ , the strengths of the different frequency components are normalized to the maximum value. The red dashed line represents the approximate boundary between  $m \sim \beta$ .

$$a(t) = a_0 e^{\frac{-iA \sin(\Omega t)}{\Omega}} e^{(-\frac{\kappa}{2} - i\omega_0)t}. \quad (\text{S32})$$

Next, we express the oscillatory factor  $e^{\frac{-iA \sin(\Omega t)}{\Omega}}$  in terms of the Bessel function. The generating function of the Bessel functions is given by:

$$e^{(\beta/2)(u-1/u)} = \sum_{m=-\infty}^{\infty} J_m(\beta) u^m, \quad (\text{S33})$$

Using this identity, we can expand the time-dependent phase factor as a sum of Bessel functions by applying on  $\beta = \frac{A}{\Omega}$  and  $u = e^{i\Omega t}$ :

$$a(t) = a_0 e^{-\frac{\kappa}{2}t} \sum_{m=-\infty}^{\infty} J_m(\beta) e^{-i(\omega_0 + m\Omega)t}. \quad (\text{S34})$$

This final expression represents the solution to the dynamics equation in terms of a series of frequency components indexed by  $m$ , weighted by the Bessel function  $J_m(\beta)$ . Here, we utilized the odd-even symmetry of the Bessel function. As mentioned in the main text, we have neglected the cavity dissipation  $\kappa$ . In Fig. S2, we show the transformation of the cavity mode distribution with respect to  $\beta$ . Theoretically,  $m$  can range from negative infinity to positive infinity. However, due to the influence of the Bessel function, the intensity of higher-order frequency components is very weak. Here, we consider the relative intensity distribution to distinguish the presence or absence of frequency components. Numerical analysis shows an effective relationship between  $m \sim [-\beta, \beta]$ .

## Supplementary Note II Floquet Cavity Frequency Comb

### A. Dynamics equation with pump tone

As mentioned in the main text, after the pump tone is injected, the essential physics of our Floquet system can be described by the following dynamics equation,

$$\dot{a}(t) = \left[ -\frac{\kappa}{2} + i(\Delta - A \cos(\Omega t)) \right] a(t) + \sqrt{\kappa_e} a_{\text{in}}. \quad (\text{S35})$$

Here, consistent with the main text,  $\Delta = \omega_p - \omega_0$  represents the detuning of the pump tone,  $\kappa_e$  denotes the external dissipation, and  $a_{\text{in}}$  represents the externally injected photons. Similarly, to simplify this equation by eliminating the explicit time dependence in the oscillatory term  $A \cos(\Omega t)$ , we introduce a transformation that factors out the time-dependent drive,

$$a(t) = e^{-\frac{iA \sin(\Omega t)}{\Omega}} c(t). \quad (\text{S36})$$

Substituting this expression into the dynamics equation, we obtain:

$$\dot{c}(t) = \left( -\frac{\kappa}{2} + i\Delta \right) c(t) + \sqrt{\kappa_e} a_{\text{in}} e^{\frac{iA \sin(\Omega t)}{\Omega}}. \quad (\text{S37})$$

The term  $e^{\frac{iA \sin(\Omega t)}{\Omega}}$  introduces a time dependence, which we will express as a sum over Bessel functions:

$$e^{\frac{A}{2\Omega}(e^{i\Omega t} - e^{-i\Omega t})} = \sum_{l=-\infty}^{\infty} J_l(\beta) e^{il\Omega t}. \quad (\text{S38})$$

Substituting this into the equation for  $\dot{c}(t)$ , we obtain:

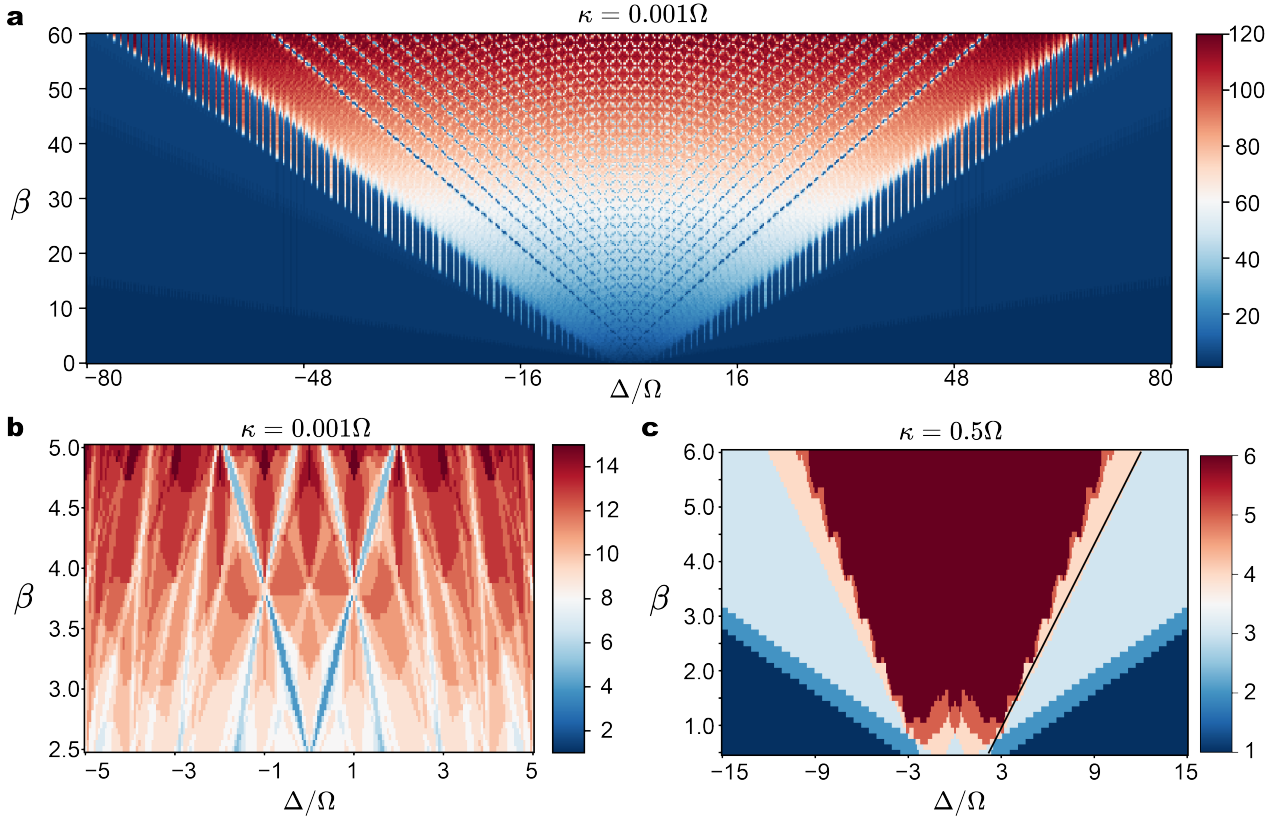

FIG. S3. The effect of  $\Delta$  and  $\beta$  is illustrated in the heatmap, where the color represents the number of valid frequency comb teeth ( $\eta > 0.1$ ). **a** The value of  $l$  is considered up to the first 160 orders, with  $\kappa = 0.001\Omega$ . **b** A partial zoom of the heatmap is shown. **c** The boundary between 3 and 4 comb teeth, where the black line represents  $\frac{\Delta}{\Omega} \simeq 1.782\beta$ , and  $\kappa = 0.5\Omega$ .

$$\dot{c}(t) = \left(-\frac{\kappa}{2} + i\Delta\right) c(t) + \sqrt{\kappa_e} a_{\text{in}} \sum_{l=-\infty}^{\infty} J_l(\beta) e^{il\Omega t}. \quad (\text{S39})$$

This is now a linear differential equation for  $c(t)$  with a driving term expressed in terms of Bessel functions. The solution to this equation is

$$c(t) = \sqrt{\kappa_e} a_{\text{in}} \sum_{l=-\infty}^{\infty} \frac{J_l(\beta) e^{il\Omega t}}{il\Omega + \frac{\kappa}{2} - i\Delta}. \quad (\text{S40})$$

Next, We substitute Eq. S40 into Eq. S36, obtaining the complete expression for  $a(t)$ ,

$$a(t) = e^{-\frac{iA \sin(\Omega t)}{\Omega}} \sqrt{\kappa_e} a_{\text{in}} \sum_{l=-\infty}^{\infty} \frac{J_l(\beta)}{il\Omega + \frac{\kappa}{2} - i\Delta} e^{il\Omega t}. \quad (\text{S41})$$

To further consider the time-dependent effects on the frequency components, we expand  $e^{-\frac{iA \sin(\Omega t)}{\Omega}}$  as a sum of Bessel functions. This gives the final expression for  $a(t)$ :

$$a(t) = \sqrt{\kappa_e} a_{\text{in}} \sum_{m=-\infty}^{\infty} \sum_{l=-\infty}^{\infty} \frac{J_l(\beta) J_{m-l}(-\beta)}{il\Omega + \frac{\kappa}{2} - i\Delta} e^{im\Omega t}. \quad (\text{S42})$$

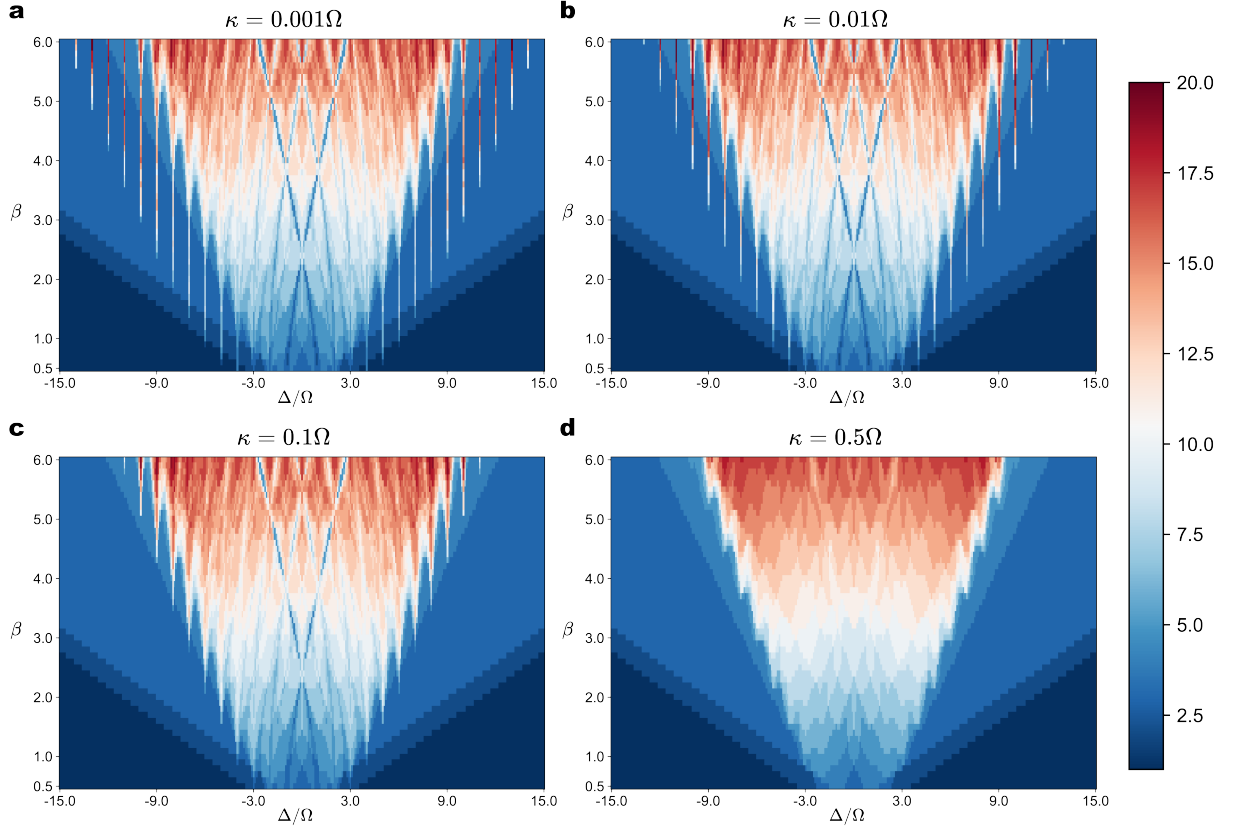

FIG. S4. The number of valid frequency comb teeth with different  $\kappa$  is illustrated in the heatmap, where the color represents the number of effective frequency comb teeth ( $\eta > 0.1$ ). The value of  $l$  is considered up to the first 50 orders. **a**  $\kappa = 0.001\Omega$ . **b**  $\kappa = 0.01\Omega$ . **c**  $\kappa = 0.1\Omega$ . **d**  $\kappa = 0.5\Omega$ .

Finally, we return to the laboratory frame and the solution for  $a(t)$  becomes

$$a(t) = \sqrt{\kappa_e} a_{\text{in}} \sum_{m=-\infty}^{\infty} \sum_{l=-\infty}^{\infty} \frac{J_l(\beta) J_{m-l}(-\beta)}{il\Omega + \frac{\kappa}{2} - i\Delta} e^{im\Omega t} e^{-i(\omega_0 + \Delta)t}. \quad (\text{S43})$$

This final expression represents the time evolution of the system's amplitude in the lab frame. It shows how the pump tone is transformed into a sum over various modes, each weighted by a Bessel function and modified by the system's parameters. We discuss in the rotating frame of the cavity frequency  $\omega_0$ , omitting the  $e^{-i\omega_0 t}$  term, in order to more clearly analyze the effects of detuning. Thus, we have  $a(t) = \sum_{m=-\infty}^{\infty} a_m e^{im\Omega t}$ , where  $a_m = \sqrt{\kappa_e} a_{\text{in}} \sum_{l=-\infty}^{\infty} \frac{J_l(\beta) J_{m-l}(-\beta)}{il\Omega + \frac{\kappa}{2} - i\Delta} e^{-i\Delta t}$ . For  $\Delta = 0$ , the distribution of  $a_m$  is nearly consistent with the Floquet cavity frequency distribution, and the effective frequency comb span is approximately  $[-\beta\Omega, \beta\Omega]$ .

To further analyze the effects of  $\Delta$  and  $\beta$  on frequency comb generation, we define the relative intensity as  $\eta = \frac{|a_m|}{\max |a_m|}$ . Fig. S3a shows the number of valid frequency comb teeth ( $\eta > 0.1$ ) versus  $\Delta$  and  $\beta$ . We observe that, due to the Bessel function's similarity to decaying cosine functions, the number of frequency comb teeth does not follow a strictly linear dependence on  $\beta$ , but instead exhibits periodic fluctuations. Similarly, changes in  $\Delta$  lead to corresponding match of different  $l$ , and the number are also influenced by the periodic-like behavior. Fig. S3b shows the local details. Additionally, numerical analysis indicates that the range of  $\Delta$  depends on  $\beta$ . As shown in Fig. S3c, for the boundary between 3 and 4 comb teeth,  $\frac{\Delta}{\Omega} \simeq 1.782\beta$ . An approximate reference is that the range of  $\Delta$  is  $-2\beta\Omega \sim 2\beta\Omega$ , as mentioned in the main text.

Notably, when  $\Delta = k\Omega$  (where  $k = 0, 1, 2, \dots$ ), local dips are observed, particularly when  $\Omega \ll \kappa$ . This is due to the fact that, for  $l = k$ , the value of  $\kappa$  significantly influences  $a_m$ , resulting in additional comb teeth near the pump tone. Fig. S4 illustrates the impact of varying  $\kappa$ .

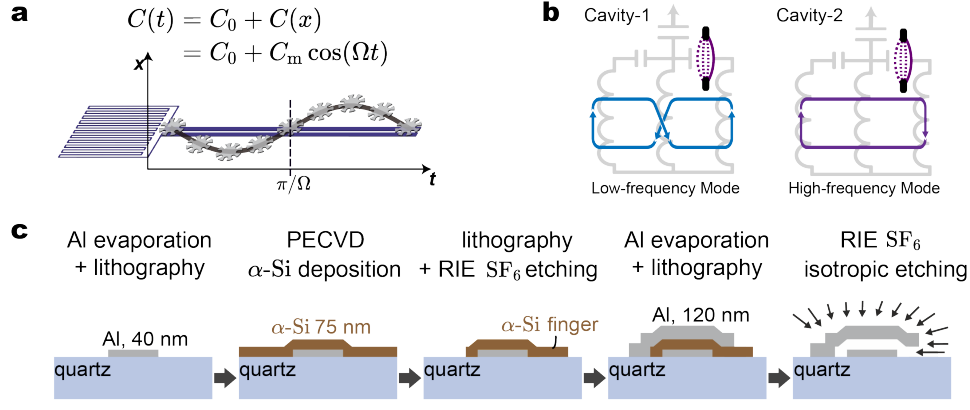

FIG. S5. **a** A schematic of the oscillator tuning the cavity frequency. **b** A schematic of the construction method for the two cavity modes is shown. The surrounding arrows indicate the direction of the current, and the ignored oscillator is replaced by a capacitor. **c** Simplified description of the fabrication process.

## B. Input-output theory

As mentioned in the main text, before constructing the frequency comb, we characterized the Floquet sidebands by measuring the reflection coefficient. This can naturally be derived from Eq. S43, where  $\Delta = \omega_p - \omega_0$ , with  $\omega_p$  no longer being a single stable pump tone but rather a set of swept-frequency signals,  $\omega_p = \omega_{\text{scan}}$ . Combined with the input-output relation:

$$a_{\text{in}}(t) = a_{\text{out}}(t) + \sqrt{\kappa_e} a(t), \quad (\text{S44})$$

we can get the reflection coefficient:

$$R = 1 - \sqrt{\kappa_e} \frac{\langle a(t) \rangle}{\langle a_{\text{in}}(t) \rangle}. \quad (\text{S45})$$

Then we substitute Eq. S43,

$$R = 1 - \kappa_e \sum_{m=-\infty}^{\infty} \sum_{l=-\infty}^{\infty} \frac{J_l(\beta) J_{m-l}(-\beta)}{il\Omega + \kappa/2 - i\Delta} \langle e^{im\Omega t} \rangle. \quad (\text{S46})$$

In the main text, the reflection coefficient is acquired using a network analyzer. The data fitting employs S46, utilizing free parameter fitting, with each frequency point averaged over a 0.1s span.

## Supplementary Note III Microwave Optomechanical Device and Characterization

### A. Sample fabrication

The device under study is based on a design similar to that described in [2, 3]. It consists of three meandering microstrip inductors, in combination with drums and stray capacitances from the meanders, which together support two microwave eigenmodes, or “cavities”. A detailed description of the microwave functionalities can be found in the Supplementary Information of Ref. [2]. The schematic of how the mechanical oscillator modulates the cavity frequency is shown in Fig. S5a. And the current flow of the two cavity modes at their respective resonance frequencies is shown in Fig. S5b.

Fabrication begins with a quartz substrate, onto which the inductors, external coupler, bottom electrodes of each drum, connecting pads, and ground planes are defined using standard electron lithography. The patterning process employs a PMMA copolymer stack and resist, followed by 40 nm of aluminum deposition via electron-beam evaporation

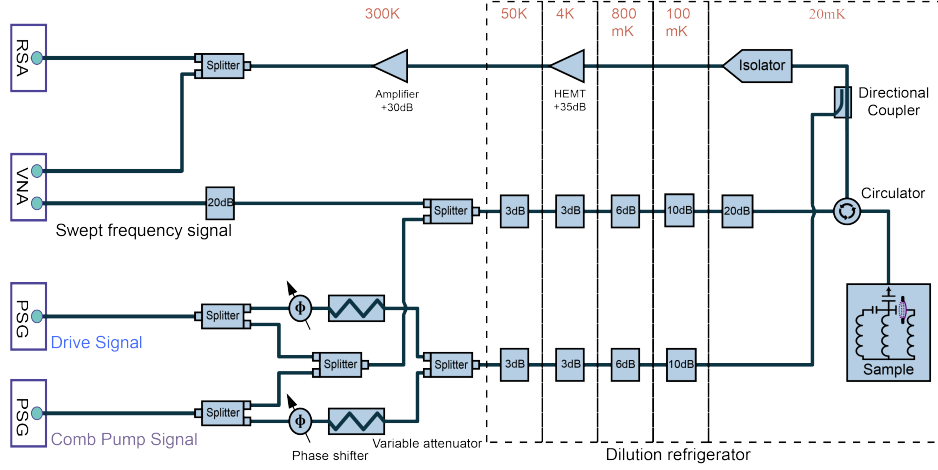

FIG. S6. Experimental setup. The sample is replaced by an equivalent effective circuit model. Blue sideband signal is injected to drive the mechanical oscillator, while another pump signal is directly used to construct the frequency comb. Heterodyne reflection readout is adopted to observe frequency comb formation.

(Fig. S5c). A 75 nm sacrificial layer of amorphous silicon is then deposited using PECVD, patterned with ma-N 2403 negative-tone resist, and etched by RIE  $\text{SF}_6$  plasma. The final step of lithography defines the 120 nm-thick aluminum drumheads.

Following dicing of the substrate into  $4 \times 4$  mm chips, the sacrificial layer is removed using isotropic RIE  $\text{SF}_6$  plasma etching, leaving a vacuum gap of approximately 80 nm. For measurements, the device is microbonded to a metallic holder, which is then sealed within a cryostat.

## B. Detailed experimental setup

Detailed cryogenic setup, as well as room temperature microwave devices are presented in Fig. S6. Attenuators in the input channels are used to reduce background noise. Circulator, isolator and directional couplers help to avoid back reflections. Network analyzer (VNA, ROHDE&SCHWARZ ZNB 20) is mainly used for preliminary characterization. Spectrum Analyzer (RSA, ROHDE&SCHWARZ FSV) is used for more specific spectrum detection, including both frequency and time domain features. Signal components involved in the experiment includes microwave range resonant frequency of the cavity, and signal generator (PSG, SINOLINK SLFS0218F) emitted drive and pump signal.

## C. Parameter characterization

As mentioned in the main text, when we neglect additional mechanical oscillators, the Hamiltonian of the total optomechanical system can be expressed as,

$$H_{\text{sys}} = \sum_{j=1,2} [\hbar\omega_{c_j} \hat{a}_j^\dagger \hat{a}_j + \hbar g_{0j} \hat{a}_j^\dagger \hat{a}_j (\hat{b} + \hat{b}^\dagger)] + \hbar\omega_m \hat{b}^\dagger \hat{b}. \quad (\text{S47})$$

where  $\omega_{c_j}$  represents two cavity's intrinsic frequency and the subscripts 1 and 2 are used to distinguish between the two different cavities.  $\omega_m$  represents the first mechanical resonant frequency, and the coefficient  $g_{0j}$  represents the single photon coupling strength between the  $j$ -th cavity and oscillator. Besides,  $a_j$  ( $a_j^\dagger$ ) and  $b$  ( $b^\dagger$ ) represent the annihilation (creation) operators for the  $j$ -th cavity and the mechanical mode, respectively.

The basic parameter characterization is obtained by separately considering the isolated optomechanical tests for each cavity interacting with the mechanical oscillator. Fig. S7a and b refer to the unpumped reflection of cavity-1 and cavity-2, respectively, which characterize the resonant frequency and damping rate. The detection is performed using the VNA. At this point that we are considering the emitted output field from the cavity, we have to split the cavity energy loss to the internal and external losses, which occur at the respective rates  $\kappa_i$  and  $\kappa_e$ , and sum up to  $\kappa = \kappa_i + \kappa_e$ .

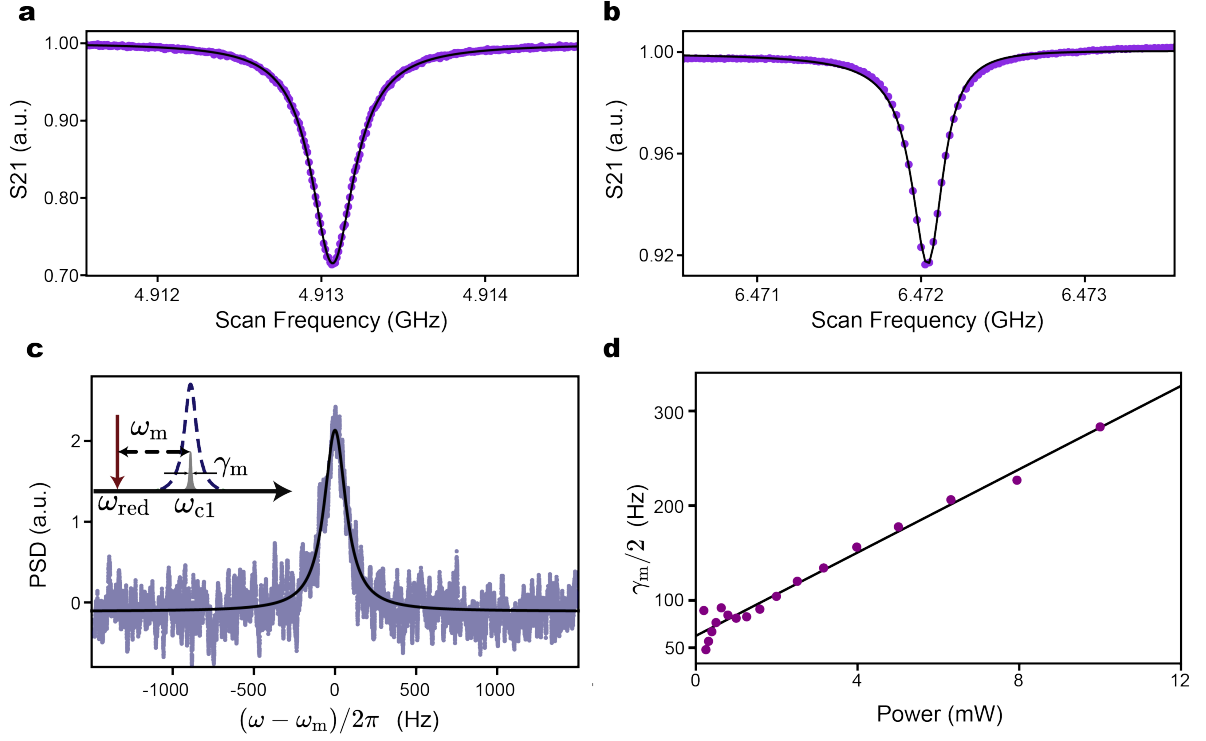

FIG. S7. Parameter characterization. Measured reflection of the microwave cavity-1 at **a** and cavity-2 at **b**. The purple dots and black solid lines denote the experimental spectrum and the corresponding circle fit, respectively. **c** Purple dots show the noise power spectrum of the thermomechanical motion. The mechanical motion is detected by applying a red-detuned microwave drive at  $\omega_{\text{red}}$ . The solid line indicates a Lorentzian fit of the mechanical resonance. The inset shows a measurement schematic in frequency-domain. The red arrow denotes a red-detuned microwave drive, the black-dashed line denotes the microwave resonance of cavity-1, and the gray shaded Lorentzian curve denotes the anti-Stokes sideband signal. **d** Dependence of half of the linewidth of the mechanical oscillator on power

The sideband-cooling situation, where the pump is set at the frequency  $\omega_{\text{red}} = \omega_{c,j} - \omega_m$ , is the basis for most calibrations. Here we utilize cavity-1 to characterize the mechanical oscillator. In the good-cavity limit, and if the optical damping due to the coherent tone  $\gamma_{\text{opt}} \ll \kappa$ , the output spectrum  $S_{\text{out}}$  after amplification with gain  $\mathcal{G}$  satisfies,

$$\frac{S_{\text{out}}[\omega]}{\mathcal{G}} = \frac{4\kappa_e}{\kappa} n_c^T + \frac{\kappa_e}{\kappa} \frac{\gamma_{\text{opt}} \gamma_{\text{eff}}}{\omega^2 + \gamma_{\text{eff}}^2/4} (n_m - 2n_c^T) + n_{\text{add}}, \quad (\text{S48})$$

The number of thermal photons  $n_c^T$  represents the classical cavity noise, while  $\gamma_{\text{opt}}$  is the effective optomechanical damping rate, and  $\gamma_{\text{eff}} = \gamma_m + \gamma_{\text{opt}}$ . Additionally,  $n_m$  refers to the number of thermal phonons, and  $n_{\text{add}}$  represents the background noise level due to amplifier added noise. The anti-Stokes sideband induced by red-detuned microwave pump reveals a mechanical spectrum measured using a spectrum analyzer, as shown in Fig. S7c. As is well-known, the optomechanical damping rate  $\gamma_{\text{opt}}$  can be written as,

$$\gamma_{\text{opt}} = \frac{4g_0^2 \bar{n}_{\text{cav}}}{\kappa}, \quad (\text{S49})$$

where the  $\bar{n}_{\text{cav}}$  is the cavity photon number under a coherent tone, which is proportional to generator power  $P_{\text{red}}$ . Therefore,  $\gamma_{\text{eff}}$  is linearly related to  $P_{\text{red}}$  with a proportionality constant  $\mathcal{K}$ ,

$$\gamma_{\text{eff}} = \mathcal{K} P_{\text{red}} + \gamma_m. \quad (\text{S50})$$

We perform a linear fit to the experimentally determined  $\gamma_{\text{eff}}$  as a function of the generator power, as shown in Fig. S7d.

Exact single photon coupling strength can be derived from comparing spectrum of the thermomechanical sideband with the spectrum of a reliable calibration tone under reliable temperature, where thermomechanical sideband is

thermally determined. The calibration is set to be slightly detuned from  $\omega_{c,j} + \omega_m$ , and outside the mechanical linewidth. Taking calibration tone as a reference, the single photon coupling strengths can be concludes as,

$$g_{0,j}^2 = \frac{r}{2n_m} \left( \frac{\kappa}{\kappa_e} \right)^2 \left( \omega_m^2 + \frac{\kappa^2}{2} \right) \frac{P_{\text{side}}}{P_{\text{cali}}}. \quad (\text{S51})$$

where  $r$  represents input power ration between injected calibration tone and cavity pump tone for the corresponding cases.  $P_{\text{side}}$  and  $P_{\text{cali}}$  represent the detected power of the thermomechanical sideband and calibration tone, measured at the end of the output chain by the RSA. The coupling strength test was performed at 70 mK, and we can conclude that  $g_{01} = 2\pi \times 79$  Hz and  $g_{02} = 2\pi \times 46$  Hz.

## Supplementary Note IV Self-induced oscillations by blue-detuned driving

For the excitation cavity-1, with the drive signal, we focus on the Hamiltonian of cavity-1 and the mechanical oscillator,

$$\hat{H}_{\text{drive}} = -\hbar\Delta_d \hat{a}_1^\dagger \hat{a}_1 + \hbar\omega_m \hat{b}^\dagger \hat{b} + \hbar g_{01} \hat{a}_1^\dagger \hat{a}_1 (\hat{b} + \hat{b}^\dagger). \quad (\text{S52})$$

Herr,  $\Delta_d = \omega_d - \omega_{c1}$  is the frequency detuning between the pump laser frequency  $\omega_d$  and the resonant cavity-1. For the blue-detuned regime ( $\Delta_d < 0$ ), the optomechanical damping rate  $\gamma_{\text{opt}}$  is negative. Initially, this results in an increase in the oscillator's effective temperature. As the overall damping rate  $\gamma_m + \gamma_{\text{opt}}$  becomes negative, any small initial fluctuation will grow exponentially over time, eventually reaching a steady-state regime. These are referred to as self-induced (or backaction-induced) optomechanical oscillations, where the mechanical oscillation amplitude stabilizes at a fixed value  $X_m$ . The governing dynamical equations are given by:

$$\frac{d^2 x(t)}{dt^2} + \gamma_m \frac{dx(t)}{dt} + \omega_m^2 x(t) = \frac{F(t)}{m_{\text{eff}}}, \quad (\text{S53})$$

where the radiation-pressure force  $F(t) = \frac{\hbar g_0}{x_{\text{zpf}}} |a_1(t)|^2$ , and  $m_{\text{eff}}$  is the effective mass of the mechanical oscillator,  $x_{\text{zpf}}$  represents the zero-point fluctuation of the mechanical oscillator's displacement.

Ignoring the phase term  $\phi_m$  in the assumption of the maintext, we have  $x(t) = X_m \cos(\omega_m t) + X_0$ . In steady state, we define an amplitude-dependent effective optomechanical damping rate as:

$$\gamma_{\text{opt}} = -\frac{\langle F\dot{x} \rangle}{m_{\text{eff}} \langle \dot{x}^2 \rangle}, \quad (\text{S54})$$

which represents the ratio of the time-averaged power input due to this force to the corresponding mechanical energy lost. The time-averaged radiation-pressure force determines the oscillation offset  $X_0$ , and by combining the balance condition of the overall damping rate, we obtain:

$$\begin{cases} m_{\text{eff}} \omega_m^2 X_0 = \langle F \rangle, \\ \gamma_m + \gamma_{\text{opt}} = 0. \end{cases} \quad (\text{S55})$$

For the quantum dynamical equations of  $a_1(t)$ ,

$$\dot{a}_1(t) = \left[ -\frac{\kappa_1}{2} + i \left( \Delta_d - \frac{g_{01}}{x_{\text{zpf}}} x \right) \right] a_1(t) + \sqrt{\kappa_{e1}} a_d, \quad (\text{S56})$$

where  $\kappa_1$  is the total decay rate of the cavity-1. With the ansatz, the solutin of  $a_1(t)$  in blue-sideband drive can be written in a Fourier series  $a_1(t) = e^{-i\varphi(t)} \sum_k a_k e^{ik\omega_m t}$ , with coefficients

$$a_k = \sqrt{\kappa_{e1}} a_d \frac{J_k(g_{01} X_m / x_{\text{zpf}} \omega_m)}{ik\omega_m + \frac{\kappa}{2} - i(\omega_m - g_{01} X_0 / x_{\text{zpf}})}, \quad (\text{S57})$$

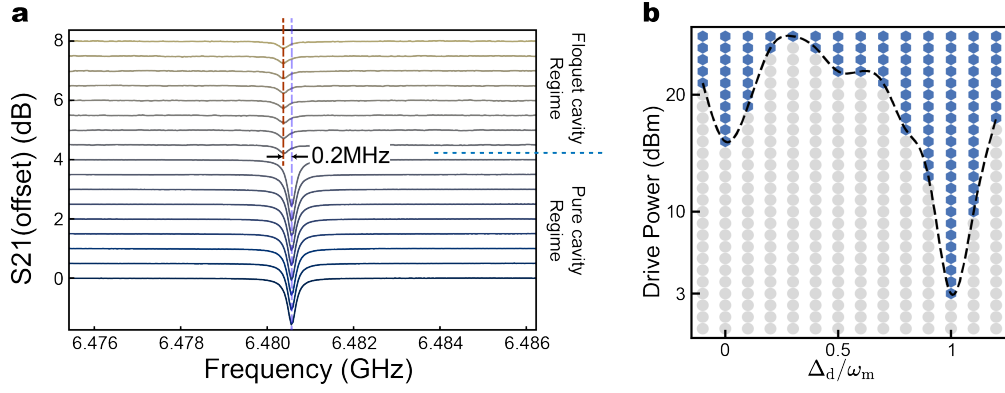

FIG. S8. **a** The shift in the center frequency of cavity-2 caused by power-dependent equilibrium position  $X_0$  is shown, with the dashed line marking the transition of the mechanical oscillator from the thermal state to self-induced oscillation. **b** The operating threshold for the mechanical oscillator transitioning from the thermal state to self-induced oscillation, where the gray points represent the thermal state. The colored points indicate the self-induced oscillation generated from optomechanical nonlinear dynamics. The black dashed line marks the dividing line between different regions.

and the global phase  $\varphi(t) = (g_{01}X_m/x_{zpf}\omega_m)\sin(\omega_mt)$ . And we can get,

$$|a(t)|^2 \approx \sum_k |a_k|^2 + 2 \sum_k \text{Re}(a_k a_{k-1}^*) \cos \Omega_m t - 2 \sum_k \text{Im}(a_k a_{k-1}^*) \sin \Omega_m t \quad (\text{S58})$$

By substituting this Fourier series into Eq. S55, we obtain the implicit equation for  $X_0$  and  $X_m$ :

$$\begin{cases} X_0 = \frac{\hbar g_{01}}{x_{zpf} m_{\text{eff}} \omega_m^2} \sum_k |a_k|^2 \\ X_m = \frac{2\hbar g_{01}}{x_{zpf} m_{\text{eff}} \omega_m \gamma_m} \text{Im} \sum_k a_k^* a_{k+1} \end{cases} \quad (\text{S59})$$

The series can be efficiently summed numerically to obtain the explicit dependence of  $X_m$  and  $X_0$  on the system parameters. This is consistent with the direct solution of Eq. S53 that balance the sine, co-sine, and constant terms, respectively,

$$\frac{d^2 x}{dt^2} + \gamma_m \frac{dx}{dt} + \omega_m^2 x = \ddot{X}_0 + \gamma_m \dot{X}_0 + \omega_m^2 X_0 + \left( \ddot{X}_m + \gamma_m \dot{X}_m \right) \cos \Omega_m t - \left( 2\dot{X}_m + \gamma_m X_m \right) \omega_m \sin \omega_m t. \quad (\text{S60})$$

This further validates the effectiveness of our assumptions and analysis. Mathematically, the onset of small-amplitude oscillations, starting from  $A = 0$ , represents a Hopf bifurcation. In this regime,  $A \propto \sqrt{|a_d|^2 - |a_d|_{\text{th}}^2}$ , where  $|a_d|_{\text{th}}^2$  is the threshold value [4–8].

## Supplementary Note V Extended Data

### A. Frequency shift caused by equilibrium position shift

As mentioned in the main text and in Note IV, changes in the mean displacement value  $X_0$  induces a shift in the central frequency of the cavity. In the main text, we incorporated this effect into  $\omega_{c2}$ . Fig. S8a shows the experimentally measured frequency shift. After entering the Floquet regime, the frequency of cavity-2 exhibits a redshift  $\delta_{c2}$  of approximately 0.2 MHz, which is much smaller than the cavity frequency. In Fig. S8a, the intrinsic frequency  $\omega_{c2}$  is 6.480 GHz, slightly deviating from the value in the main text. This discrepancy arises from measurements taken from different experimental runs of the same sample, where minor changes in the sample parameters occurred during the cooling and warming process of the dilution refrigerator.

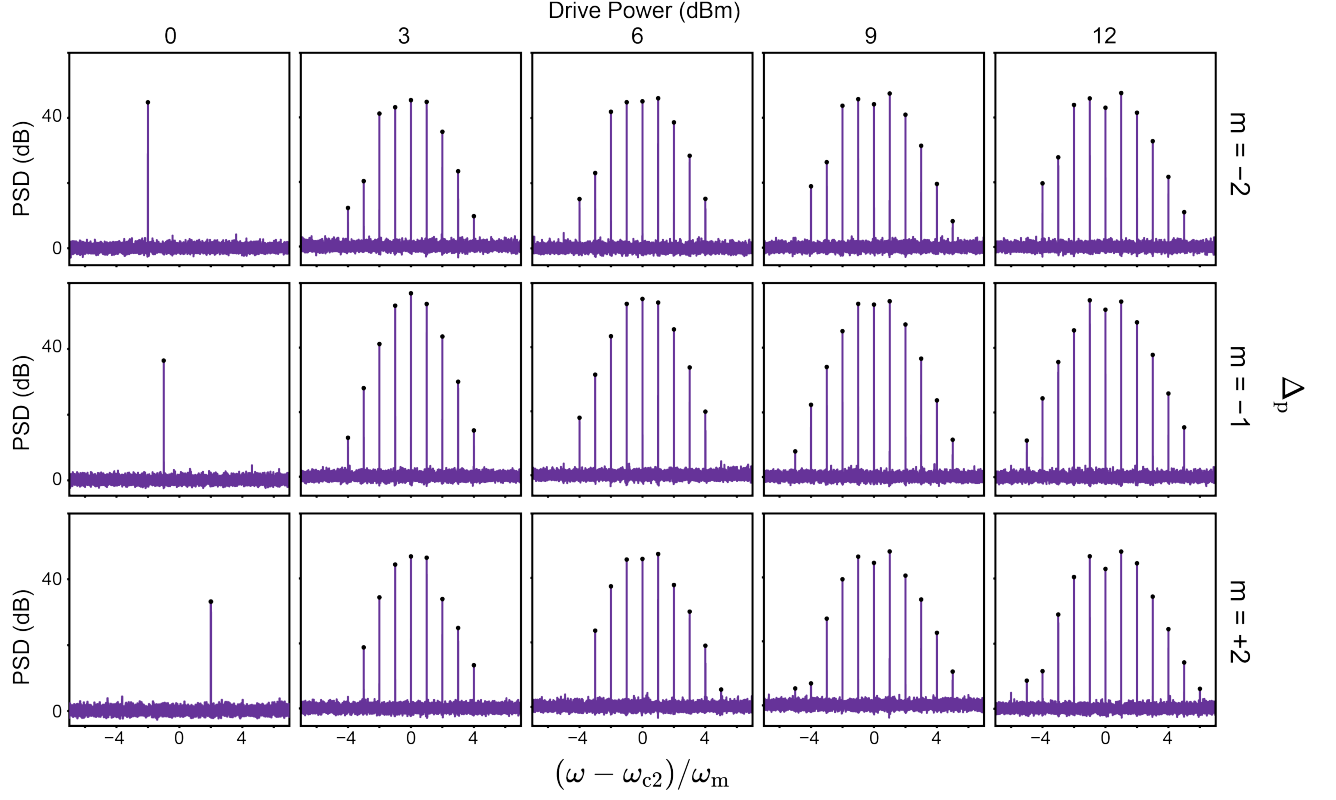

FIG. S9. Detailed formation of Floquet frequency comb for  $\Delta_p/\omega_m = -2, -1, +2$  with different drive power. All data have been baseline-corrected.

### B. The self-induced oscillation regime

We characterized the operating range of the mechanical oscillator from the thermal state to self-induced oscillation. As shown in Fig. S8b, the global minimum at the blue sideband  $\Delta_d/\omega_m \approx 1$  results from maximal frequency down-conversion, which most efficiently reduces the overall damping rate. The other local minimum of the self-induced oscillation threshold occurs near  $\Delta_d/\omega_m \approx 0$ , resulting from the largest photon flux at cavity resonance. The minimum power required for cavity-1 to drive mechanical oscillator into self-induced oscillation is  $P_d = P_{de} = 3\text{dBm}$ .

### C. Detailed Floquet Frequency Comb

We present more detailed frequency comb characteristics in Fig. S9. As mentioned in the main text, although  $\Delta_p$  can alter the relative amplitudes of the comb teeth to some extent, the overall frequency comb still distributes progressively from the cavity's intrinsic frequency toward both sides. As shown in Fig. S9, with a fixed pump power of 0 dBm, we set the pump tone at  $m = -1, 0, +1$  and demonstrated how the frequency comb evolves with varying drive power. Before reaching  $P_{de}$ , we measured pure pump tones, with the intensity differences arising from different line cancellation adjustments.

- 
- [1] Bukov, M., D'Alessio, L. & Polkovnikov, A. Universal high-frequency behavior of periodically driven systems: From dynamical stabilization to floquet engineering. *Adv. Phys.* **64**, 139–226 (2015).
  - [2] Mercier de Lépinay, L., Ockeloen-Korppi, C. F., Woolley, M. J. & Sillanpää, M. A. Quantum mechanics-free subsystem with mechanical oscillators. *Science* **372**, 625–629 (2021).
  - [3] Wang, C. *et al.* Ground-state cooling of a mechanical oscillator by a noisy environment. *Nat. Commun.* **15**, 7395 (2024).
  - [4] Aspelmeyer, M., Kippenberg, T. J. & Marquardt, F. Cavity optomechanics. *Rev. Mod. Phys.* **86**, 1391–1452 (2014).

- [5] Marquardt, F., Harris, J. G. E. & Girvin, S. M. Dynamical Multistability Induced by Radiation Pressure in High-Finesse Micromechanical Optical Cavities. *Phys. Rev. Lett.* **96**, 103901 (2006).
- [6] Ludwig, M., Kubala, B. & Marquardt, F. The optomechanical instability in the quantum regime. *New J. Phys.* **10**, 095013 (2008).
- [7] Miri, M.-A. Optomechanical frequency combs. *New J. Phys.* **20**, 043013 (2018).
- [8] Krause, A. G. *et al.* Nonlinear radiation pressure dynamics in an optomechanical crystal. *Phys. Rev. Lett.* **115**, 233601 (2015).
